# Supplementary material for: ESC: Erasing Space Concept for Knowledge Deletion
Source: arXiv:2504.02199 source file (2025-04-03)
Supplement: Supplementary file 1 [file tab_RN50.tex]

\begin{table}[tb]
\caption{Accuracy and RS performance using ResNet-50.}
\label{tab:rn50}
\centering

\resizebox{\textwidth}{!}{
%{\scriptsize
\begin{tabular}{lccccgg}
\toprule
\multirow{2}{*}{Method} & \multicolumn{6}{c}{CIFAR-10} \\ \cmidrule{2-7}
& $D_f(\downarrow)$ & $D_r(\uparrow)$ & $D_{ft}(\downarrow)$ & $D_{rt}(\uparrow)$ & $HM(\uparrow)$ & $HM_{\text{t}}(\uparrow)$ \\
\midrule
Original & 99.90 & 99.76 & 98.70 & 96.47 & 0.20 & 2.57 \\
\methodname (Ours) & 9.26 & 92.99 & 8.80 & 89.02 & 91.85 & 90.10 \\
\refinemethod (Ours) & 0.00 & 99.75 & 0.00 & 96.64 & 99.87 & 98.29 \\
\midrule
Retrain & 0.00 & 98.63 & 0.00 & 96.27 & 99.31 & 98.10 \\
\bottomrule
\end{tabular}

\begin{tabular}{ccccgg}
\toprule
\multicolumn{6}{c}{CIFAR-10$-RS$} \\ \cmidrule{1-6}
$D_f(\downarrow)$ & $D_r(\uparrow)$ & $D_{ft}(\downarrow)$ & $D_{rt}(\uparrow)$ & $HM(\uparrow)$ & $HM_{\text{t}}(\uparrow)$ \\
\midrule
96.52 & 98.20 & 96.33 & 99.78 & 6.72 & 7.08 \\
30.56 & 98.76 & 29.40 & 95.02 & 81.54 & 81.01 \\
90.28 & 99.48 & 89.80 & 95.66 & 17.71 & 18.43 \\
 \midrule
91.14 & 98.06 & 91.40 & 95.24 & 16.25 & 15.78 \\   
\bottomrule
\end{tabular}
}

\resizebox{\textwidth}{!}{
%{\scriptsize
\begin{tabular}{lccccgg}
\toprule
\multirow{2}{*}{Method} & \multicolumn{6}{c}{CIFAR-100} \\ \cmidrule{2-7}
& $D_f(\downarrow)$ & $D_r(\uparrow)$ & $D_{ft}(\downarrow)$ & $D_{rt}(\uparrow)$ & $HM(\uparrow)$ & $HM_{\text{t}}(\uparrow)$ \\
\midrule
Original & 96.98 & 96.49 & 80.30 & 83.70 & 5.86 & 31.89 \\
\methodname (Ours) & 0.06 & 87.10 & 0.20 & 74.73 & 93.08 & 85.46 \\
\refinemethod (Ours) & 0.00 & 94.44 & 0.00 & 81.79 & 97.14 & 89.98 \\
\midrule
Retrain & 0.00 & 92.89 & 0.00 & 82.36 & 96.31 & 90.33 \\
\bottomrule
\end{tabular}

\begin{tabular}{ccccgg}
\toprule
\multicolumn{6}{c}{CIFAR-100$-RS$} \\ \cmidrule{1-6}
$D_f(\downarrow)$ & $D_r(\uparrow)$ & $D_{ft}(\downarrow)$ & $D_{rt}(\uparrow)$ & $HM(\uparrow)$ & $HM_{\text{t}}(\uparrow)$ \\
\midrule
95.30 & 94.33 & 79.80 & 82.19 & 8.95 & 32.43 \\
0.10 & 81.18 & 0.10 & 70.89 & 89.57 & 82.93\\
21.94 & 94.03 & 18.40 & 82.13 & 85.30 & 81.86 \\
 \midrule
62.12 & 91.21 & 62.50 & 81.66 & 53.53 & 51.40 \\   
\bottomrule
\end{tabular}
}

\vspace{-5mm}
\end{table}
